# Supplementary material for: AerialVLN: Vision-and-Language Navigation for UAVs
Source: arXiv:2308.06735 source file (2023-08-13)
Supplement: Supplementary file 1 [file A.SupplementalMaterial.tex]

This supplementary document is organised as follows:

\begin{itemize}

    \item \textit{Section \ref{sec: dataset} Dataset}, which presents the data collection process in details.
    We also present the thumbnails of each scenario, which show the rich diversity of our dataset.

    \item \textit{Section \ref{sec: experimental details} Experimental Details}, which describes the training details. 
    
    We also provide several videos to show the agent navigating procedures.

\end{itemize}

\section{Dataset}
\label{sec: dataset}

This section presents more details on data collection and the analysis of our AerialVLN dataset.

\subsection{Data Collection}
\label{sec:DataCollection}

The collection process of AerialVLN dataset includes the following steps: path generation (step 1 to 6), instruction collection (step 7 to 11) and finalisation process (step 12), as shown in Figure \ref{fig:dataset_collection_flow}.

\begin{figure*}[h]
    \centering
    \includegraphics[width=\textwidth]{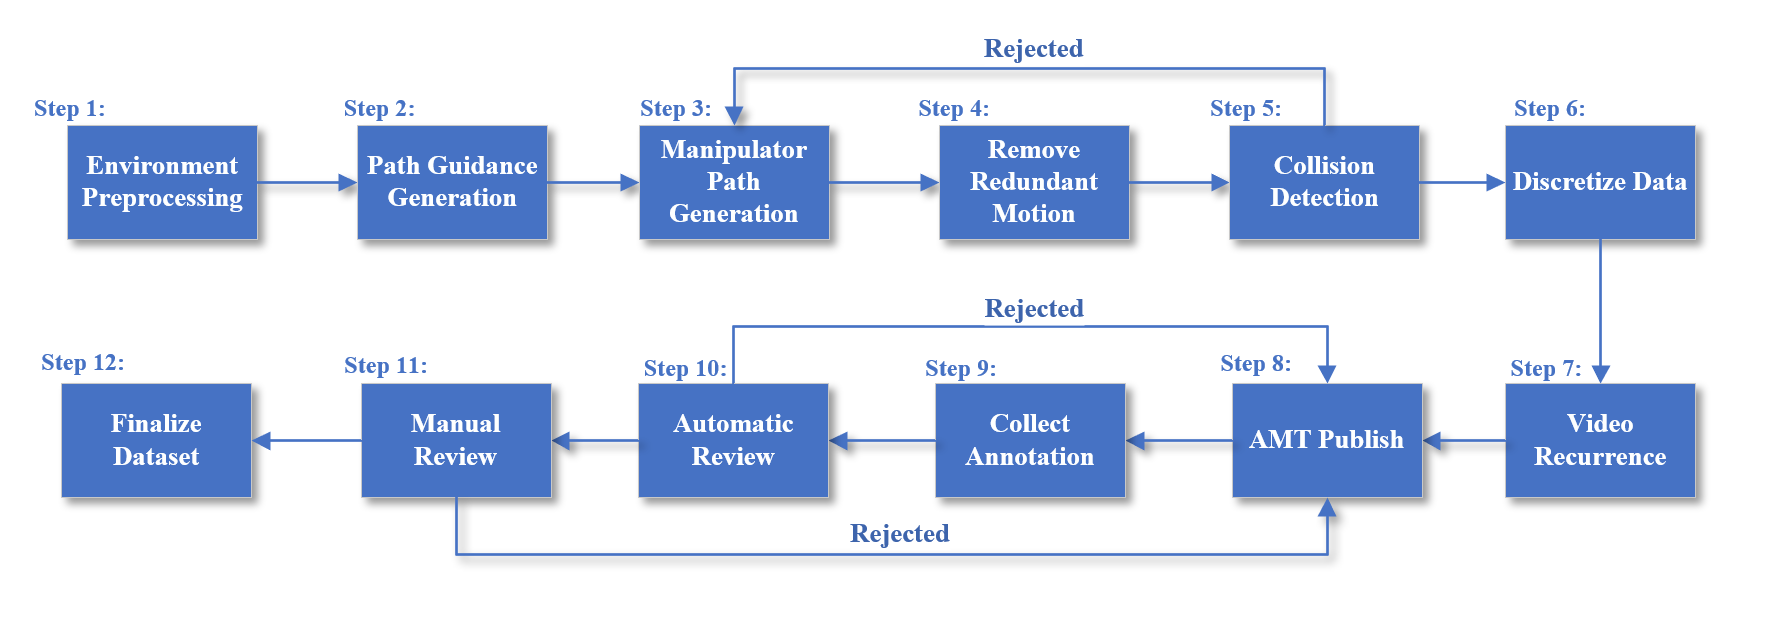}
    \caption{
    Data collection process.
    The collection process of AerialVLN dataset includes: path generation (step 1 to 6), instruction collection (step 7 to 11) and finalisation process (step 12)
    }
    \label{fig:dataset_collection_flow}
\end{figure*}

\noindent\textbf{Path generation} 
Our simulator and environments are based on Unreal Engine 4 and the AirSim plugin, which enables operators to control agents in 3D continuous environments.
Considering that the manipulation of a multirotor requires specialised knowledge, we employ experienced manipulators with AOPA licenses.
Similar to the multirotor navigation in real life, our manipulators are provided with mission guidance via showing orientation information for the necessary bypasses and middle points that they have to reach.
Path collection interface are shown in Figure \ref{fig:path_collection}.
During flying, our recording program automatically records operations of these expert manipulators every 1 millisecond, including timestamp, the position and orientation (in quaternion format) of the aerial vehicles and the input history from the keyboard.

\begin{figure*}
    \centering
    \includegraphics[width=\linewidth]{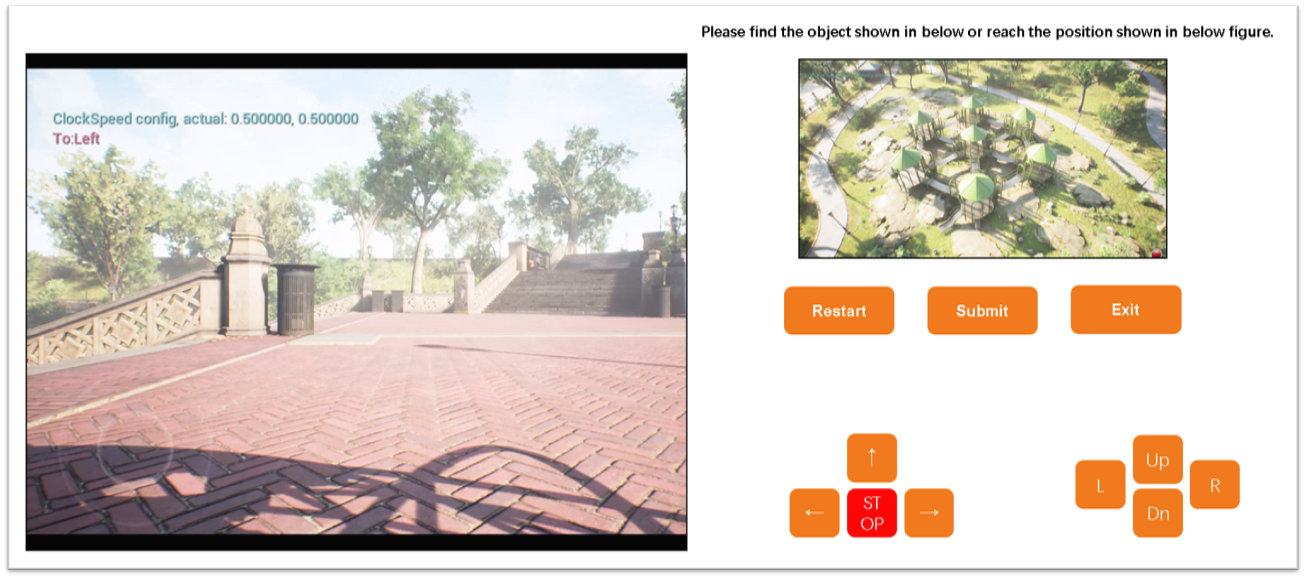}
    \caption{Path collection interface. Annotators are provided with goal image. Each annotator is allowed to pre-explore the given scene. }
    \label{fig:path_collection}
\end{figure*}

As mentioned in Section 5.1 of our main manuscript, there are redundant motions in the raw navigation records, such as looking around for seeking the next landmark and potential route. These are considered as ``noise''  actions for training models.
Thus, we merge these rotation motions. For example, if the manipulator turns 45 degrees left and then 15 degrees right heading straight, it will turn out to be turning 30 degrees left and heading straight.
Manipulators are required to avoid any collisions, just like flying in our real world, where collisions will lead to serious consequences.
When a collision is detected during flying, it will be marked as a \textit{mission failure}.

\vspace{2mm}

\noindent\textbf{Path Discretisation} 
We set 5 meters as one horizontal movement unit, 2 meters as one vertical movement unit and 15 degrees as one rotation unit. 
Take \textit{Move Forward} as an example, our discretization policy is: compare the current position $P_t=[x_t, y_t, z_t, p_t, r_t, y'_t]$ to its following manipulator's position $P^m_{t'}$, if the difference between $P^m_{t'}$ and $P_t$ is no less than a movement unit (5 meters in this example), the next action of the discretised trajectory will be \textit{Move Forward}.
{All the discretisation process is done by a program in an automatic fashion.}
Figure \ref{fig:data_descretize_compare} shows the comparison of trajectory before (red curve) and after discretization  (blue curve).
We can see that the discretisation is highly close to the continuous flying path, and the slight difference caused by discretisation is neglectable.
\begin{figure*}[!tb]
    \centering
    \includegraphics[width=\linewidth]{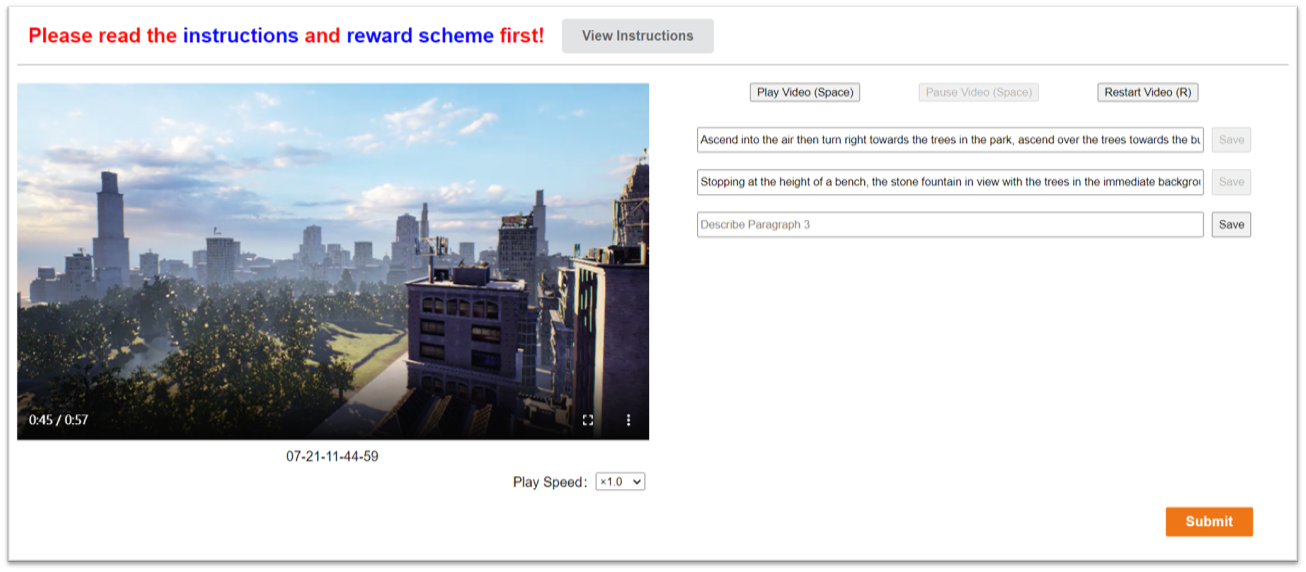}
    \caption{Instruction collection interface on AMT. Annotators are allowed to play, pause or replay the video and add descriptions.}
    \label{fig:AMT_interface}
\end{figure*}
\begin{figure}[htb]
    \centering
    \begin{subfigure}[b]{0.49\linewidth}
        \includegraphics[width=\linewidth]{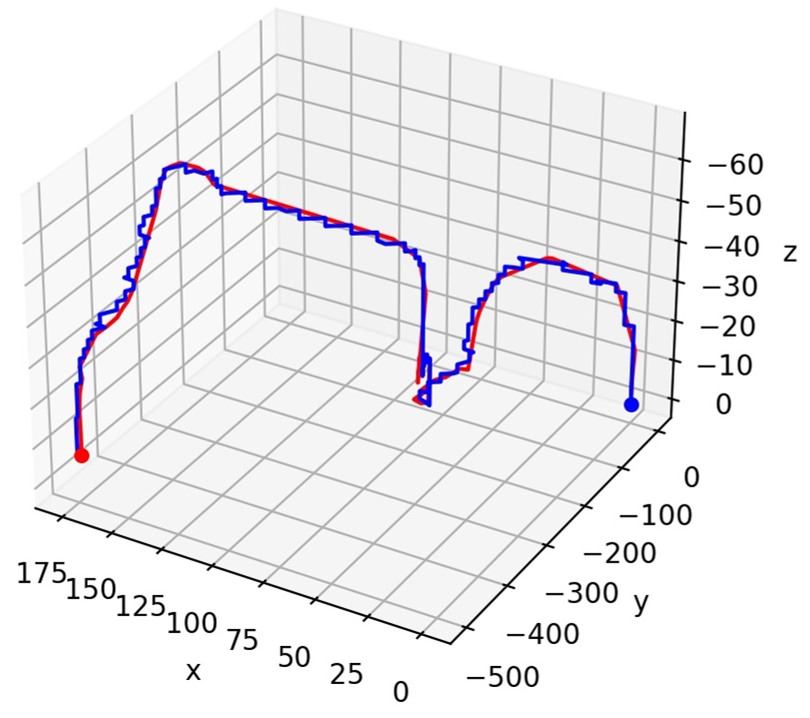}
        \label{fig:subfigure1}
    \end{subfigure}
    \begin{subfigure}[b]{0.49\linewidth}
        \includegraphics[width=\linewidth]{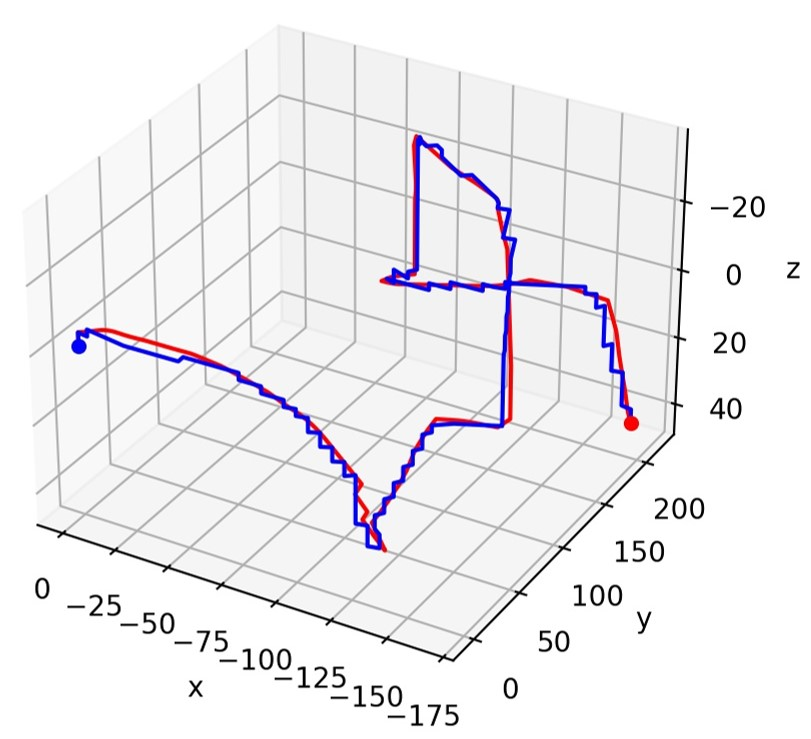}
        \label{fig:subfigure2}
    \end{subfigure}
    \caption{The trajectories before (red) and after (blue) discretization are very similar. }
    \label{fig:data_descretize_compare}
\end{figure}

\vspace{2mm}

\noindent\textbf{Instruction collection}
As illustrated in Figure \ref{fig:dataset_collection_flow}, \textit{success} paths obtained from manipulators will be used to reproduce flying videos for annotators on Amazon Mechanical Turk (AMT) to collect instructions.
Figure \ref{fig:AMT_interface} shows the annotation interface.
The annotators are requested to describe the multirotor's movements in everyday English. 
At least 3 lines of description are required before submission.
Eventually, 2,444 workers participated in our task, spending 5074.51 hours in total, with an average of 596.22 seconds per assignment.

\begin{figure}[!tb]
\centering
\begin{tcolorbox}[arc=0mm,auto outer arc, colframe=blue, colback=white, leftrule=1pt, rightrule=1pt, toprule=1pt, bottomrule=1pt]
\includegraphics[width=\linewidth]{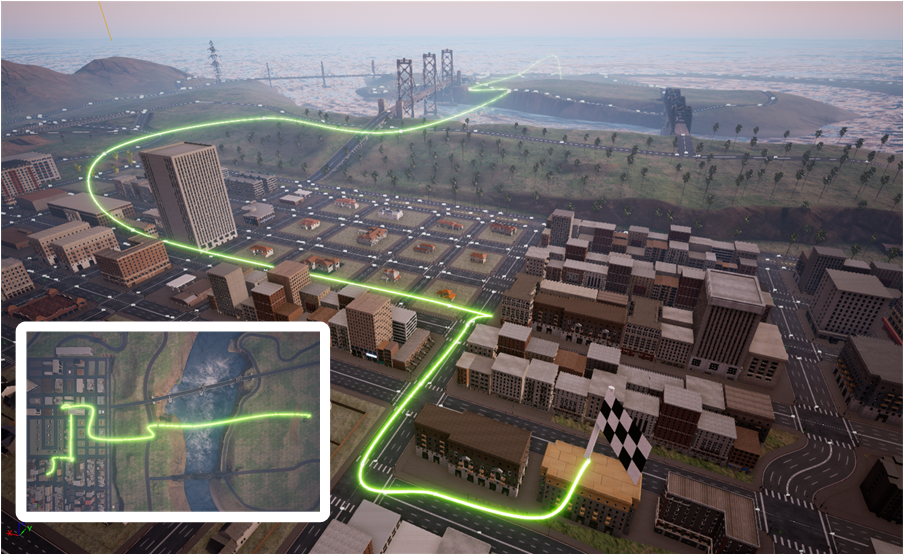}
\caption*{\textbf{Instruction}: Ascend and turn to the riverside, fly parallel to the bridge over the river. Turn right and cross the road, march forward to the top of the largest white building. Descend and turn left towards the intersection, head straight down this street until the drone reaches the next intersection. Turn right and pass a brown building, land on the top of an adjacent orange building.}
\end{tcolorbox}
\caption{Examples of AerialVLN dataset.
The green line shows the trajectory of the ground truth path. 
}
\label{fig:example of dataset}
\end{figure}

\vspace{2mm}

\noindent\textbf{Review Policy}
As mentioned in Section 5.1 of the main manuscript, we employ another group of workers to verify the quality of collected instructions and to ensure instructions are consistent with flying procedures in videos. 
The details of the instruction review policy are as follows:

\begin{itemize}
    \setlength{\itemsep}{2pt}
    \setlength{\parsep}{0pt}
    \setlength{\parskip}{0pt}
    \item Each specific motion like \textit{Ascend}, \textit{Descend} must be mentioned in the instruction; At least one landmark is required as reference when describing a steering action like \textit{Turn Left}, \textit{Turn Right}. 
    \item In the description of the destination, instructions should include specific actions like \textit{Stop} or \textit{Land} corresponding to a landmark as a signal to finish. 
    \item Spelling and grammar check is conducted.
    \item Ambiguous instructions will be re-annotated. For example, ``...turn right at the building...'', in which if ``the building'' is found to cause ambiguity, we require re-annotation.
\end{itemize}

Figure \ref{fig:example of dataset} presents one example of instruction after data reviewing process.

\vspace{2mm}

\noindent\textbf{Dataset Finalisation}
Finally, following the same partition as R2R~\cite{DBLP:conf/cvpr/AndersonWTB0S0G18} and Reverie~\cite{DBLP:conf/cvpr/QiW0WWSH20}, we split data into train, validation seen, validation unseen, test set according to the ratio 6 : 1 : 1 : 2.
Each split includes all main scenario types, such as downtown city, countryside and factory.

\vspace{2mm}

\subsection{Dataset ethical principles}
As mentioned in Section \ref{sec:DataCollection}, another group of workers are employed to verify the quality of collected instructions.
The instructions are only allowed to describe the trajectories of drones. Any instructions that are irrelevant to drone missions or not consistent with flying procedures will be re-annotated or discarded.
Therefore, the AerialVLN dataset does not contain any other information such as personal sensitive data from which others could identify individuals, either directly or indirectly.

To benefit the research community, we allow free access to researchers for academic purposes only, after signing the terms of use agreement form. 
We will also develop a website and evaluation server for future researchers to explore AerialVLN dataset and evaluate their results.

\subsection{More Data Analysis}

We present the word frequency in the form of sunburst graph in Figure \ref{fig:sunburst}, which indicates the word preference when giving a command to multirotor.
Instructions are read from the centre outwards and the longer the arc, the higher the word frequency. It shows that people prefer to use ``turn'', ``fly'', and ``go'' at the beginning of instructions. On the second ring, we note that ``turn'' is most frequently followed by ``left'' and ``right'', and they occupy the similar percentage. For verbs ``move'' and ``go'', they are usually followed by ``forward''. 
\begin{figure}[!tb]
    \centering
    \includegraphics[width=\linewidth]{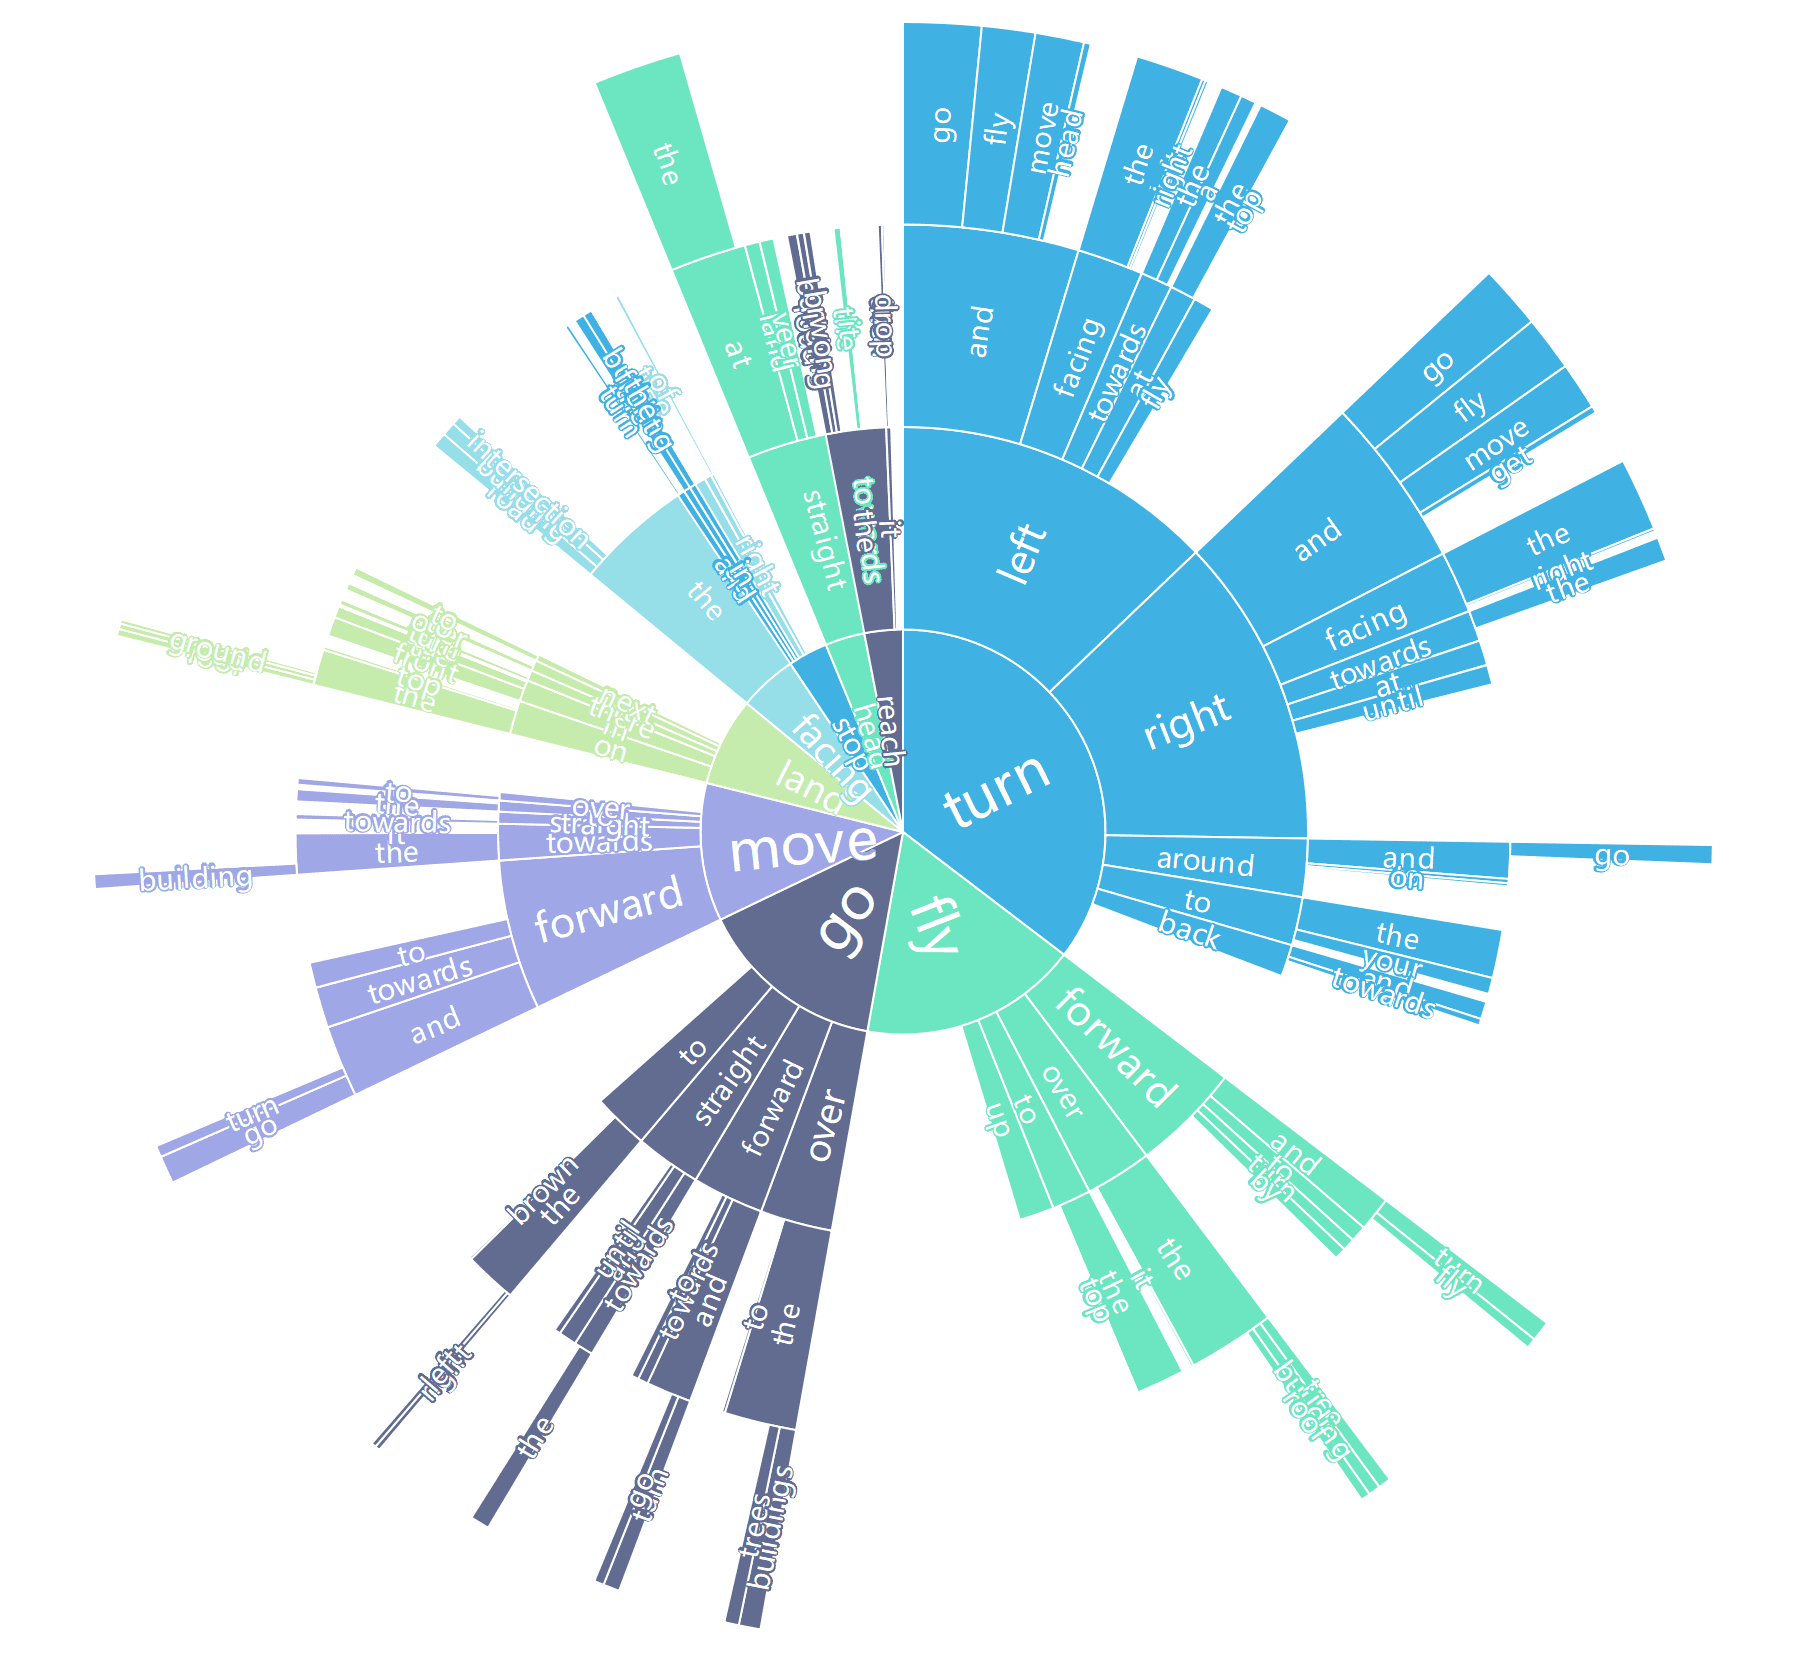}
    \caption{Distribution of navigation instructions based on their first four words. Instructions are read from the centre outwards. Arc lengths are proportional to the number of instructions containing each word. White areas represent words with individual contributions too small to show.}
    \label{fig:sunburst}
\end{figure}

In Figure \ref{fig:scenes}, we present scenario samples of all environments. It shows that our AirVLN dataset has a rich diversity, covering a large diversity of scenarios, including downtown city (day and night, modern and last century style), countryside, factory, container port, etc. 
Such diversity could significantly narrow the gap between simulator and real-world applications.
We also provide some videos of ground truth path flying in the supplement, where Video 1 and 2 show the flying procedure on the train set. 
RGB signal, depth signal of each step and corresponding trajectory are presented from left to right, respectively, and instruction is at the bottom.

{In Table \ref{tab:example_instruction}, we present some randomly sampled instructions, which shows our dataset has diverse language phenomena.}

\begin{figure*}[htb]
    \centering
    \includegraphics[width=\linewidth]{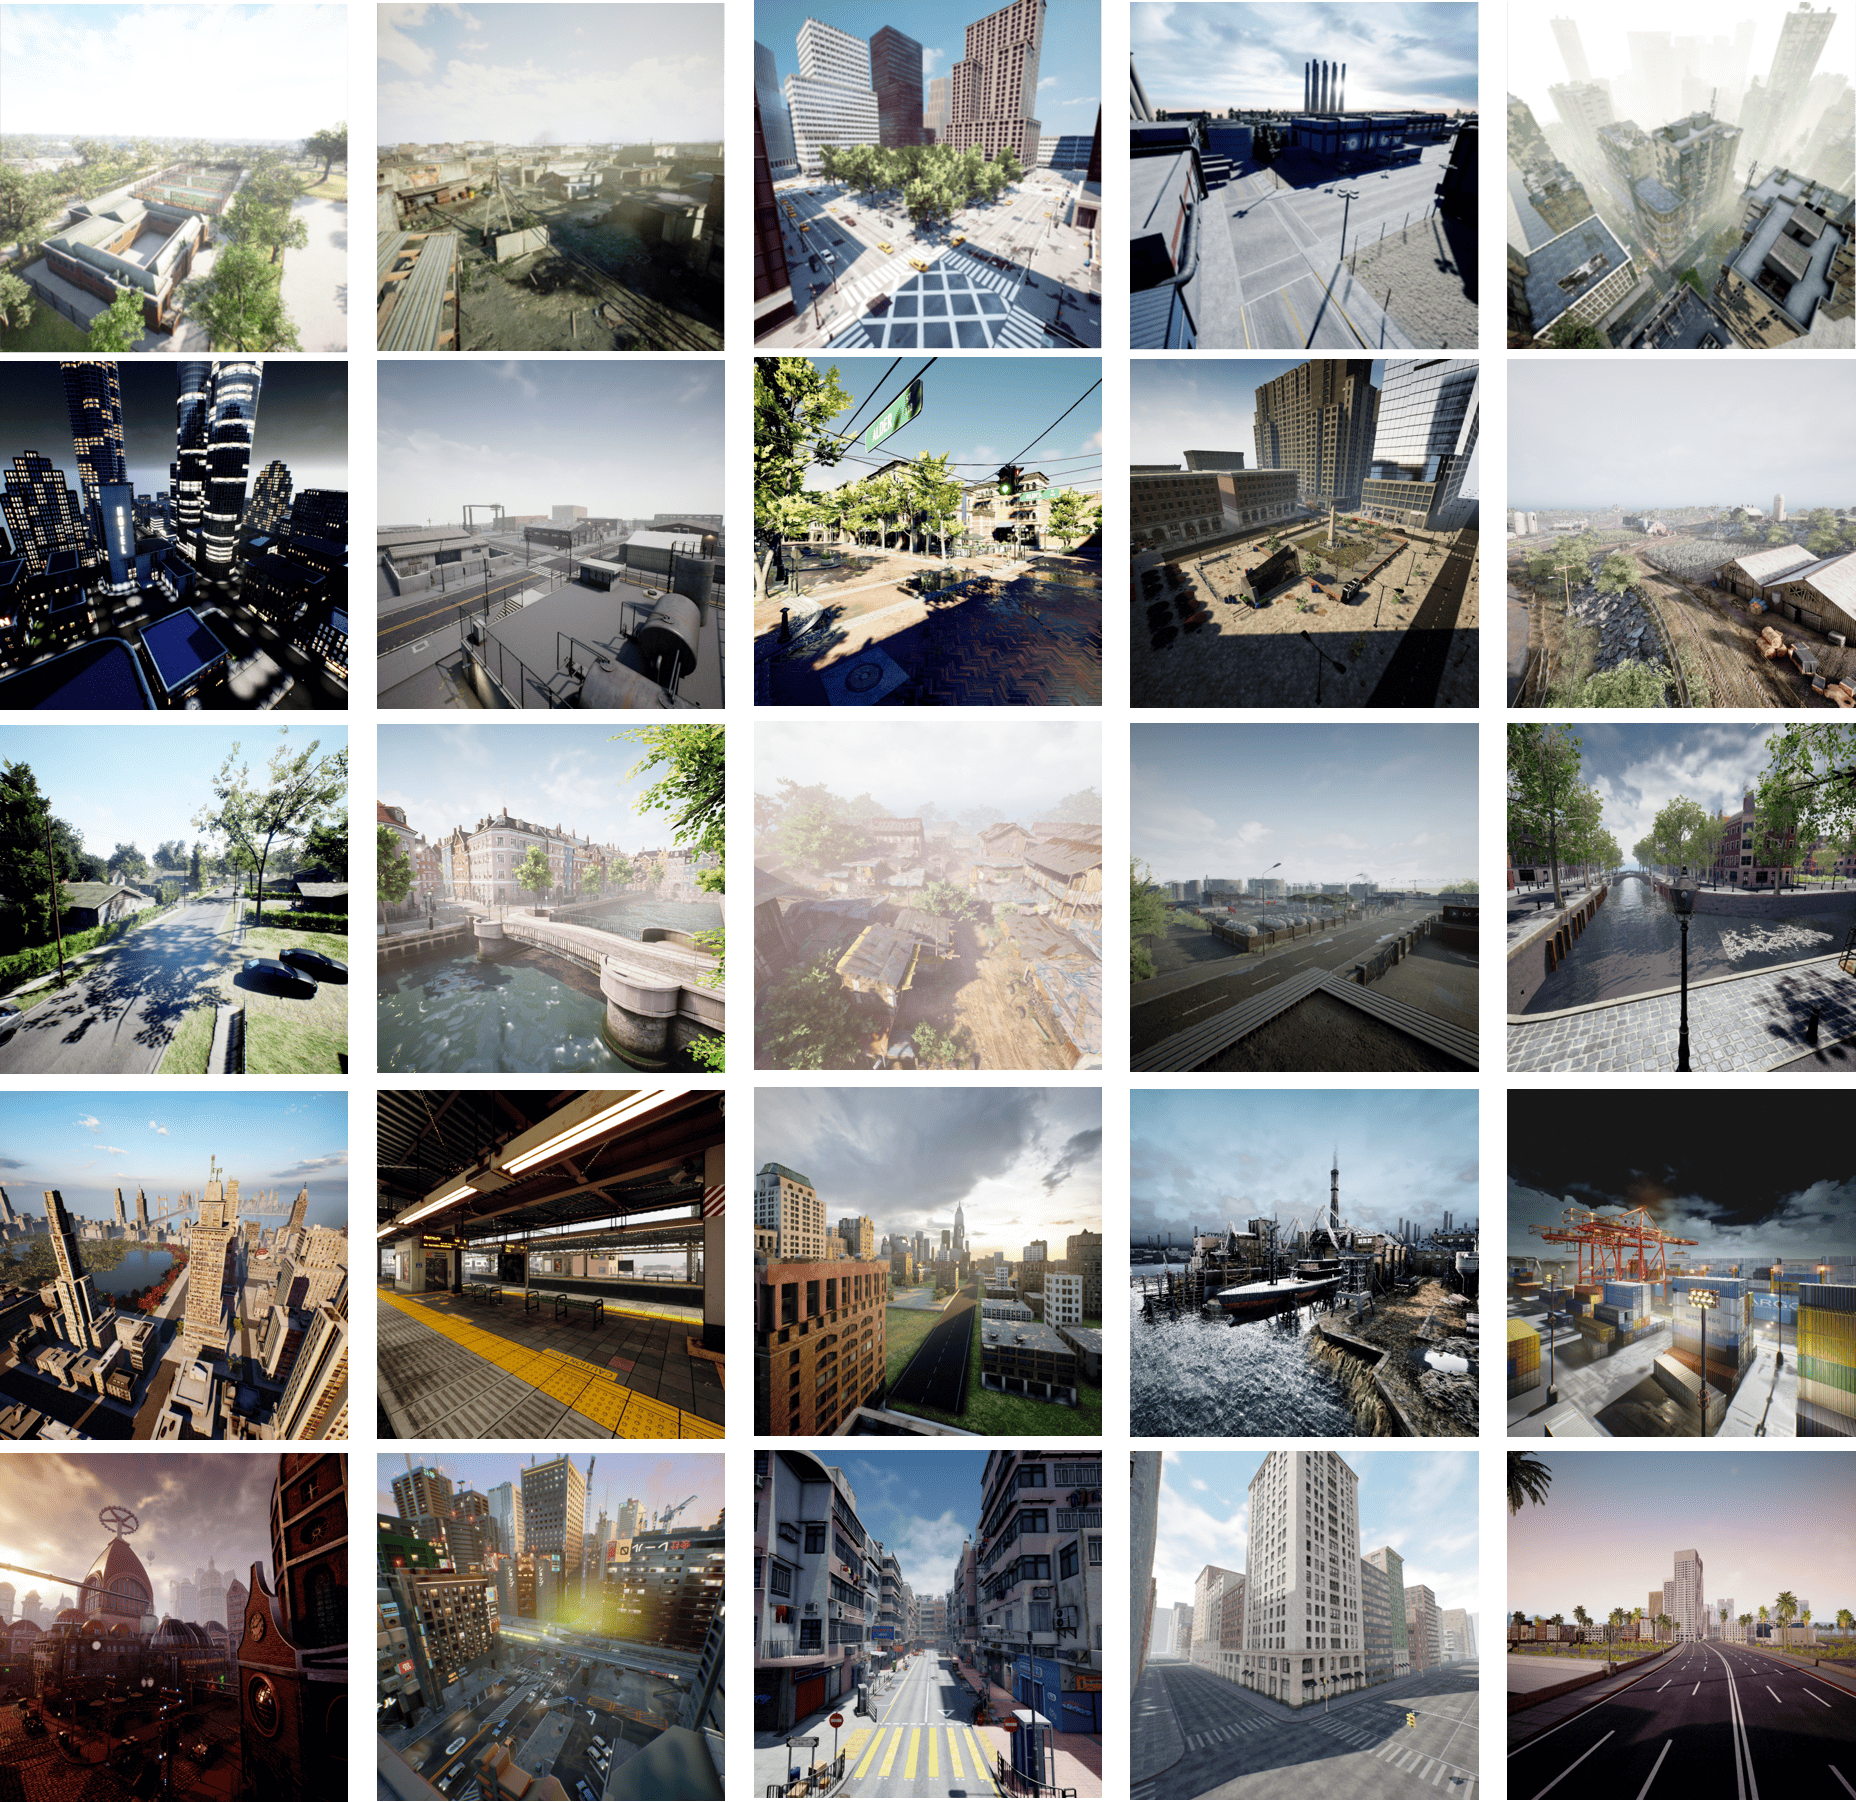}
    \caption{Scene samples of all environments in our AerialVLN dataset}
    \label{fig:scenes}
\end{figure*}

\section{Experimental Details}
\label{sec: experimental details}

In this section, we present training details of our baseline models and the visualisation of navigation results.

\subsection{Action Sampling Baseline}
This baseline samples actions according to action distribution in the training split, which is a more reasonable random baseline, comparing to pure random agent which sample each action in equal possibility.
We present the action sampling distribution of AerialVLN and AerialVLN-S dataset for researcher to reproduce.
The action distribution of the AerialVLN training set is $50\%$ forward, $10\%$ turn-left, $10\%$ turn-right, $13\%$ ascend, $12\%$ descend, $2\%$ move-left, $2\%$ move-right, $1\%$ stop.
The action distribution of the AerialVLN-S training set is $44\%$ forward, $15\%$ turn-left, $15\%$ turn-right, $11\%$ ascend, $10\%$ descend, $2\%$ move-left, $2\%$ move-right, $1\%$ stop.

\subsection{Human Performance Baseline}
{
As mentioned in Section 6.2 in the main manuscript, we present human performance in the AerialVLN task. 
The human baseline is completed by professional pilots with AOPA (Aircraft Owners and Pilots Association) Licence.
Pilots can only operate agents to conduct actions in action space, as shown in Section 4. 
The episode ends when the human pilot clicks \textit{STOP} button or step limitation is reached.
Following R2R~\cite{DBLP:conf/cvpr/AndersonWTB0S0G18}, one-third of the test split is human tested. 
As shown in Figure \ref{fig:human_baseline_interface}, pilots fly with first-person-view RGB, depth images and language instructions.
}

\begin{figure*}
    \centering
    \includegraphics[width=\linewidth]{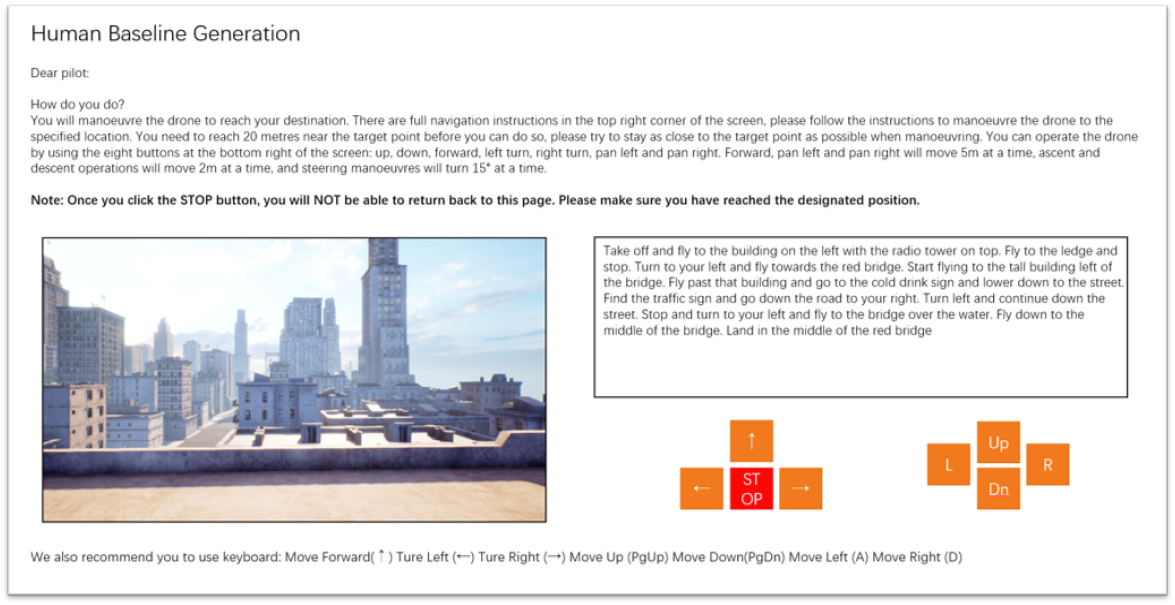}
    \caption{Human baseline generation interface. Pilots are expected to manipulate drones to reach the destination with given buttons (actions) and language instructions. Once the STOP button is pressed, the episode is considered irreversibly ended.}
    \label{fig:human_baseline_interface}
\end{figure*}

\subsection{Training Details}
We trained the baseline models on one node with 4 NVIDIA A100 GPUs. 
The learning rate is set to 0.00025.
The batch size is set to 4, the maximum length of input tokens is 300 and the maximum number of actions is 500 steps.
Then, the seq2seq model training takes about 7 hours and the CMA model takes about 18 hours for each DAgger iteration.

\vspace{2mm}

\textbf{Environment Parallelism} To accelerate training and evaluation process, we employ two parallelism method: environment parallelism and agent parallelism. 
Typically, we employ 8 environments in parallel and 2 agents for each environment during training process, and render speed varies between 400 to 1600 FPS according to the size of environment.
In addition, future work can also explore node parallelism for further acceleration.

\subsection{Visualisation of Results}
In addition to the visualisation of trajectories of the LAG model in Figure 6 of our main manuscript, here we present a successful example  of the CMA model as shown in Figure \ref{fig:cma_success_example}.
We can see that the agent can act as indicated by the instruction ``Lift up above the tall building...''  to avoid collisions.
The last several landing actions are also consistent with the instruction ``... lower down to the park behind it...". 
Moreover, we provide two videos (Video 3 and 4) in the supplements to show the completed navigating procedures of the Seq2Seq and CMA baselines.

\begin{figure*}[htb]
    \centering
    \includegraphics[width=\linewidth]{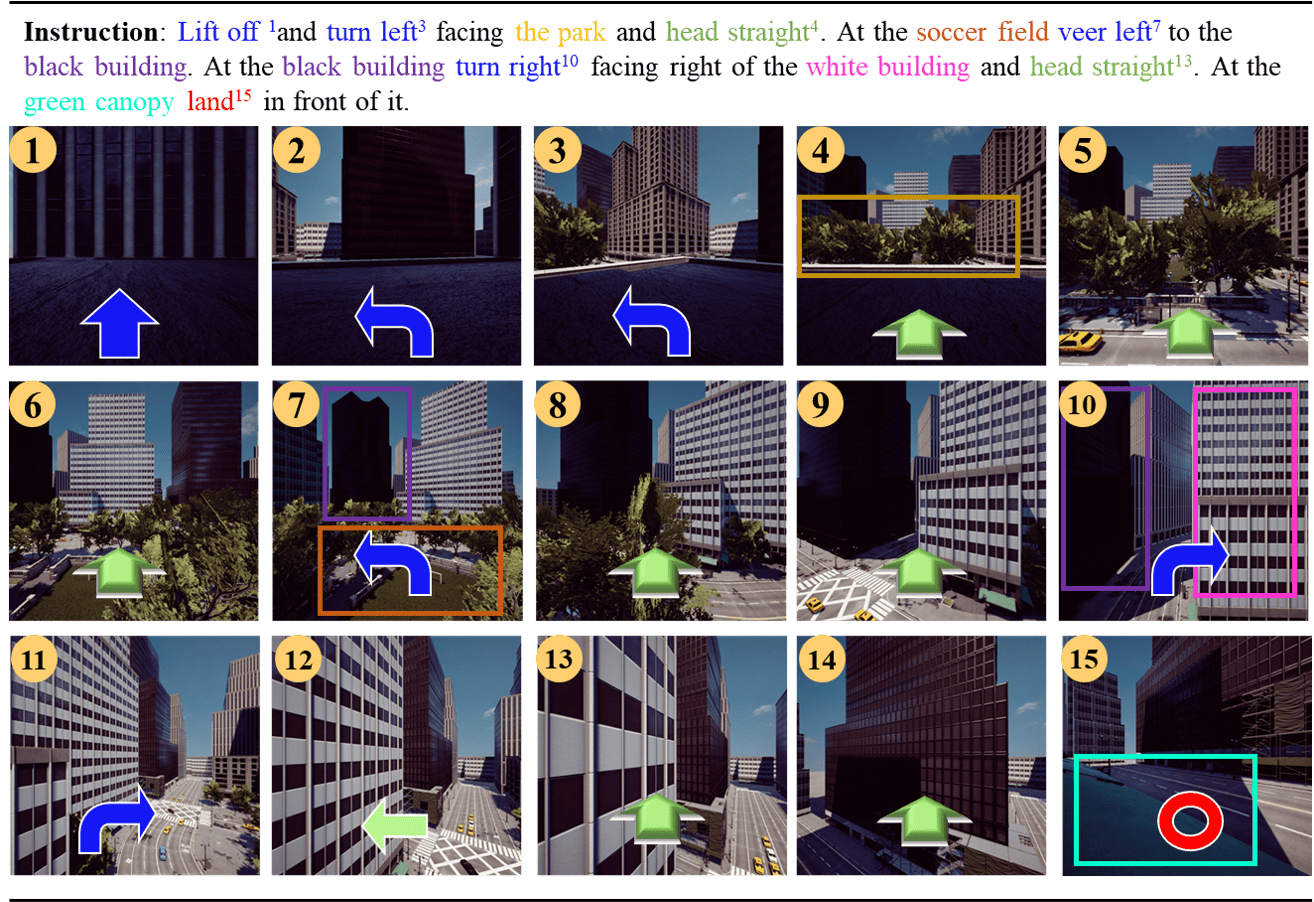}
    \caption{Visualisation of a success navigation predicted by the baseline model CMA. Green arrows indicate horizontal movement motions (Move Forward, Move Left/Right), and blue arrows denote vertical motion and horizontal rotation (yaw). The final red circle denotes the Stop action. We highlight aligned landmarks by coloured bounding boxes in images and words in the instruction using the same colour. The superscript of words denotes the index of the corresponding action in images}
    \label{fig:cma_success_example}
\end{figure*}

\subsection{DAgger Algorithm}

As mentioned in Section 6.2.2 of our main manuscript, we apply Dataset Aggregation (DAgger) policy towards Seq2Seq and CMA baselines.
Firstly, it will collect a dataset $D$ to train a model that could best mimics the expert's behaviour. 
Then at iteration $n$, it uses the last best model to collect more trajectories $D_n$ into the dataset $D$.
DAgger training scheme allows data aggregation from all iterations 1 to $n$. Each iteration optimises based on all pass trajectory data.

\subsection{Further failure analysis}
We randomly selected and visualised 100 episodes. 
We find that: 42\% of failures were caused by collision with objects; 
20\% were caused by stopping too early; 
14\% were due to the model’s inability to recognise directions; 
8\% were distracted by similar but incorrect landmarks; 
4\% passed the target location but not stopped; 
the remaining 12\% did not show obvious failure patterns.
We also provides illustration of top 3 failure case, shown in Video 3-5.

\subsection{Difference between LAG and LAW.}
The waypoints in LAW are manually annotated in R2R dataset with language supervision. The distance between two waypoints of LAW is usually around 10 units. [29]
By contrast, there are no such waypoints in our dataset and thus LAG generates the path returning to the ground-truth trajectory based on the basic unit environment and no fine-grain language alignment.

\begin{table*}
    \centering
    \begin{tabularx}{\textwidth}{X}
    \toprule

    - Take off and turn right. Move forward towards the road and beside the trees and reach the snakes stop. Now move forward and over the tree and reach the lake beside the road and turn little right. Now move forward over the trees and reach the patio table front side. Now move forward and turn little left and reach the base ball ground and land there. \\
    
    - Take off and turn right and fly forward. Fly over the trees and turn little left and fly over the roads. Now fly down and fly towards the road. Rise up and fly towards the pond and fly down towards the pathway. Now turn right and fly up and fly over the pond we just mentioned and white fountai. Then cross the road and fly down towards the restaurant. Now fly up and fly over the baseball ground and fly down towards the baseball pitch. \\
    
    - Lift off and turn right facing the intersection with a cone in it and head straight. Before the lake veer right to the lake. At the lake veer right to the overpass and head straight. Veer right to the right baseball diamond and land there. \\

    \hrule
    \vspace{3mm}

    - Taking off under the bridge. Turning left and flying by the side of the gold building. Turning left after passing it and going down toward the main street. Flying up to the grey building. Turning right and going down facing the green building. Landing on the green building. \\

    - Take off and turn left. Move forward to the road and towards the building beside the road. Then turn left to go over to the building. Now go forward and go over to the building terrace and turn left. Now go forward to the building and get down to reach the road beside the car and go over to the building and turn right. Now go forward and towards the green building to arrive at the edge of the corner and turn left. Now go forward and go over to the building to arrive at the green building terrace on the land. \\

     - Take off under the bridge and turn left on the street. Then turn left and go up in between two buildings until it reaches the top. Go straight-forward and down next to the train bridge. Turn left and go all the way down the street, veer right in front of a blue car. Go up again to the top of nearest building and turn right in front of an antenna that was on top of that building. Looking around continuing to go forward. Go straight to the green building and up to its roof. \\

    \hrule
    \vspace{3mm}

    % Done Checking

    - Take off and then turn right. After that, fly forward. Fly down until above the first roof and then fly forward. Fly down until above the street and then turn left after that fly forward. Turn right towards a red car when near an intersection and then fly forward. Pass by the red car and then land on the street near a concrete barricade. \\

    - Take off, turn right and drop down toward the flat, tan roofs until you can see the brown, brick building. Turn left and fly passed the yellow truck. Turn right toward the red car and crosswalk. Fly straight passed the red car. Land on the road facing a concrete slab with yellow and black lines. \\
    
    - Turn right and float down to the road. Turn left and go to the crosswalk. Turn right and proceed down the sidewalk and park by the concrete barrier on the roadside. \\

    \hrule
    \vspace{3mm}

    - Elevate the cam a little high and then turn to your left. Go straight until you reach the four-way connector. Fly to the other side of the river and then turn to your left. Then fly over the river. Once you reach the pavement go straight. Once you reach the pavements end tilt to the left side slightly. Pass over the river there you can find some stairs lay the cam on it. \\

    - Lift off and turn left 90 degrees until facing the road then head straight. Just past the first bridge on the right turn right 90 degrees and head straight. On the other side of the road turn left 90 degrees and head straight. At the last 'A' sign on the left of the road turn 45 degrees left and land in front of the steps near the deck. \\
    
    - Take off the drone and then move left. Then move forwards to the first intersection. Then take a right diversion to cross the river. And then take a left diversion and move forwards all the way down. Finally, you reach the strains on your left side. \\
     
    \bottomrule
    
    \end{tabularx}
    \caption{Randomly sampled  instructions. Each row contains 3 instructions that correspond to the same path.}
    \label{tab:example_instruction}
\end{table*}
